# Supplementary material for: CyberMentor: AI Powered Learning Tool Platform to Address Diverse Student Needs in Cybersecurity Education
Source: arXiv:2501.09709 source file (2025-01-16)
Supplement: Supplementary file 1 [file appendix.tex]

\section{Implementation Details}
\label{section:appendix}
The appendix details the CyberMentor framework's core components and their roles in cybersecurity learning, along with the methodology for RAG evaluation and the use of the LLM ReAct Agent framework to enhance decision-making through integrated reasoning and action generation.

\begin{table}[ht]
\caption{Summary of Core Components in the ``CyberMentor" Framework for Cybersecurity Learning.}
\label{tab:summary_components}
\begin{tabular}{M{1.8cm} M{6.2cm}}
\hline
\textbf{Component}  & \textbf{Function}     \\ \hline
User Interface (UI) & Enables user interaction, including query transaltion, submission and guidance retrieval.           \\ \hline
Agent               & Processes queries and delivers tailored responses using appropriate resources and tools.      \\ \hline
Knowledge Base (KB) & Provides quick access to organized and up-to-date educational content. \\ \hline
Skills Base (Tools) & Supports technical skill development through hands-on learning and problem-solving.                \\ \hline
\end{tabular}
\end{table}

\subsection{Prompt Engineering}
Prompt engineering is a fundamental technique used to enhance the performance of large language models (LLMs) by optimizing the structure and content of input prompts. Effective prompt design significantly influences the accuracy, relevance, and usefulness of the model’s output, particularly in educational contexts.

\subsection{LLM Agent}
\label{appx:agent}

\begin{figure}[ht]
\centering
\includegraphics[width=8cm]{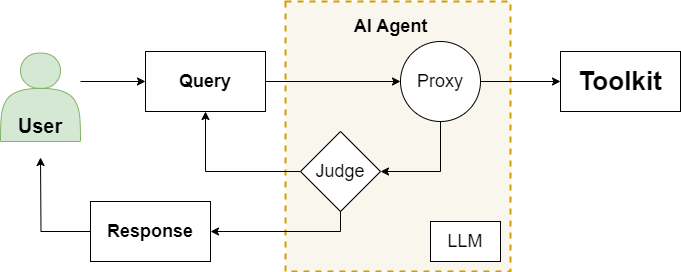}
\caption{Flowchart illustrating LLM ReAct Agent}
\label{fig:Agent}
\end{figure}

The LLM ReAct Agent is an advanced framework that integrates reasoning and action generation within large language models (LLMs). As proposed by Yao et al. \cite{yao2023reactsynergizingreasoningacting}, this framework allows LLMs to generate reasoning traces that are interleaved with task-specific actions, effectively synergizing these processes to enhance decision-making and problem-solving capabilities. Figure \ref{fig:Agent} provides a flowchart representation of the ReAct Agent, highlighting the integration of reasoning and action processes.
